# Supplementary material for: Few-photon all-optical phase rotation in a quantum-well micropillar cavity
Source: arXiv:2106.13650 ancillary file (2021-06-25)
Supplement: Supplementary file 1 [file supplementary.pdf]

# Supplementary Material: Few-photon all-optical phase rotation in a quantum-well micropillar cavity

Tintu Kuriakose,<sup>1</sup> Paul M. Walker,<sup>1,\*</sup> Toby Dowling,<sup>1</sup> Oleksandr Kyriienko,<sup>2</sup> Ivan A. Shelykh,<sup>3,4</sup> Phillipe St-Jean,<sup>5</sup> Nicola Carlon Zambon,<sup>5</sup> Aristide Lemaître,<sup>5</sup> Isabelle Sagnes,<sup>5</sup> Luc Legratiet,<sup>5</sup> Abdelmounaim Harouri,<sup>5</sup> Sylvain Ravets,<sup>5</sup> M. S. Skolnick,<sup>1,4</sup> Alberto Amo,<sup>6</sup> Jacqueline Bloch,<sup>5</sup> and D. N. Krizhanovskii<sup>1,4</sup>

<sup>1</sup>*Department of Physics and Astronomy, University of Sheffield, S3 7RH, Sheffield, UK*

<sup>2</sup>*Department of Physics and Astronomy, University of Exeter, EX4 4QL, Exeter, UK*

<sup>3</sup>*Science Institute, University of Iceland, Dunhagi 3, IS-107, Reykjavik, Iceland*

<sup>4</sup>*Department of Physics and Technology, ITMO University, St. Petersburg, 197101, Russia*

<sup>5</sup>*Centre de Nanosciences et de Nanotechnologies (C2N), 911200 Palaiseau, France*

<sup>6</sup>*Université de Lille, CNRS, Laboratoire de Physique des Lasers Atomes et Molécules (PhLAM), 59000 Lille, France*

## Supplementary Discussion 1. Device properties and measurement setup

The sample consists of a GaAs cavity containing a single 15nm  $\text{In}_{0.05}\text{Ga}_{0.95}\text{As}$  quantum well (QW) at the electric field antinode and embedded between two  $\text{Al}_{0.1}\text{Ga}_{0.9}\text{As}/\text{Al}_{0.95}\text{Ga}_{0.05}\text{As}$  Bragg mirrors. This configuration allows for strong coupling between QW excitons and photons confined by the distributed Bragg mirrors. The planar cavity was etched into an array of pillars of various sizes using inductively coupled plasma etching. Supplementary Figure 1 shows scanning electron microscope images of micropillar devices on the sample used in the experiment. The Bragg mirrors, along the pillar long axis, confine light within a wavelength-size cavity so that the optical wavevector is primarily in the longitudinal direction. Then, weaker confinement on micrometer scales in the transverse direction occurs through total internal reflection. The confinement in all three dimensions results in discrete optical modes. Supplementary Figure 1a shows pillars of the same shape and size (uppermost pillar) as pillars A and B used for the phase shift measurements (see main text). Supplementary Figure 1b shows several arrays of pillars. Each array contains pillars of different sizes. The arrays at different positions have different exciton-photon detuning allowing selection of different excitonic fraction of the polaritons.

Supplementary Figure 2 illustrates the experimental setup for making the phase measurements. The signal and control beams are combined on a beam-splitter and focused onto the micropillar using a 50x microscope objective. The transmitted light is collected by a second microscope objective. The control beam light is filtered out by a spectrometer. The signal beam polarisation component intensities are measured using avalanche photodiodes connected to a time-correlated photo-counting (TCSPC) system. The TCSPC is synchronised to the signal laser repetition using a photodiode so that signal counts appear as a peak at a well defined time whereas other counts appear as a constant background offset

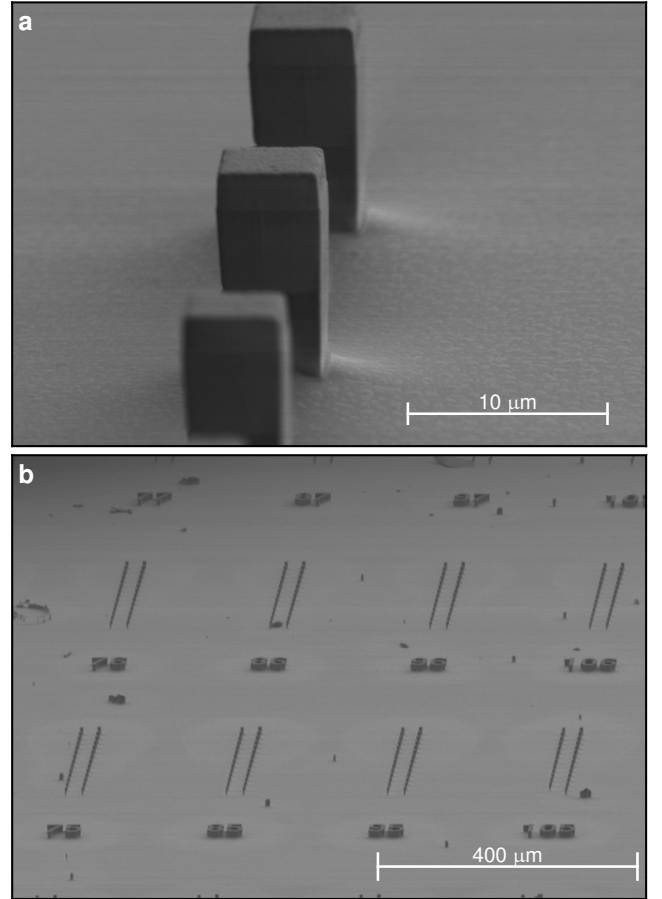

**Supplementary Figure 1.** Scanning electron microscope images of the sample at two different zoom levels.

which can be removed. The TCSPC routing also keeps track of the control beam state (on or off). See Supplementary Discussion 3 for further details of the TCSPC data collection and processing.

\* [p.m.walker@sheffield.ac.uk](mailto:p.m.walker@sheffield.ac.uk)

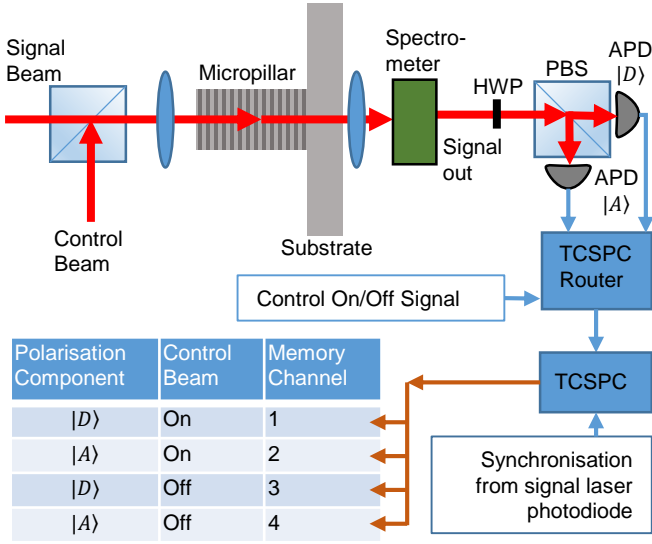

**Supplementary Figure 2.** Schematic of phase measurement apparatus. HWP and PBS are a half wave plate and polarising beam-splitter used to rotate the linear polarisation state and select the diagonal ( $|D\rangle$ ) / anti-diagonal ( $|A\rangle$ ) basis. APDs are avalanche photodiodes. TCSPC is the time-correlated single photon counting card used to measure the rate of photons arriving at the APDs.

### Supplementary Discussion 2. Nonlinear polarisation rotation

Since we deal with small nonlinear changes in the exciton and polariton frequencies compared to all other energy scales in the system (of which the smallest is the linewidth) we can solve the problem with nonlinear terms set to zero and then include the nonlinearity as a first order perturbation. We then note that the signal beam pulse lengths  $> 100$  ps are long compared to the polariton decay rate so that the optical field in the pillar can be approximated as simply following the temporal envelope of the incident pulses. Next we note that the energy separation between the control and signal states is sufficiently large compared to the laser and state linewidths that there will be negligible coupling of the signal laser to the control states. Furthermore, the signal laser has flat phase in the  $x$  direction but its phase changes sign in the  $y$  direction. Thus, it has the same symmetry as the  $E_{12}$  doublet and can excite it efficiently, but it cannot excite the  $E_{21}$  doublet since the phase flip causes its overlap with those states to cancel out. Thus, the only states relevant to the signal are the two orthogonal polarisation components comprising the  $E_{12}$  doublet. The evolution

of these can then be written as given in Eqn. (S1).

$$i \frac{\partial}{\partial t} \begin{pmatrix} u_x \\ u_y \end{pmatrix} = \mathcal{H} \begin{pmatrix} u_x \\ u_y \end{pmatrix} + \begin{pmatrix} P_x \\ P_y \end{pmatrix} e^{-i\Delta_p t}, \quad (\text{S1a})$$

$$\mathcal{H} = \begin{pmatrix} \omega_{BS} + \frac{\omega_s}{2} - i\frac{\gamma}{2} & -i\frac{\omega_Z}{2} \\ i\frac{\omega_Z}{2} & \omega_{BS} - \frac{\omega_s}{2} - i\frac{\gamma}{2} \end{pmatrix}. \quad (\text{S1b})$$

Here,  $u_x$  and  $u_y$  are the complex field amplitudes of the lower polariton branch states in two orthogonal linear polarisations. We choose a linear polarisation basis since the  $E_{12}$  doublet has finite momentum in the  $y$  direction which will cause a TE-TM frequency splitting between linear polarisations parallel and perpendicular to the momentum. We excite with a signal beam linearly polarised parallel to this momentum.  $\omega_s$  is the size of the linear polarisation splitting. Experimentally, this splitting could not be resolved in the spectra indicating that it is less than the linewidth.  $\gamma$  is the polariton FWHM linewidth.  $\Delta_p$  is the signal laser detuning from the average frequency of the two polarisation-split states.  $P_x$  and  $P_y$  are the complex amplitudes describing the incident signal beam polarisation. Since our signal beam is linearly polarised they could be written  $P_x = \cos \theta_p$ ,  $P_y = \sin \theta_p$  where  $\theta_p$  between 0 and 90 degrees is the angle of the pump beam from the +ve  $x$ -axis (see diagram in Fig. 1a of the main text) towards the +ve  $y$ -axis. The nonlinearity enters through a rigid frequency blueshift  $\omega_{BS}$  of all states and a frequency splitting  $\omega_Z$  between circularly polarised polaritons. This latter corresponds to a nonlinear effective magnetic field. The size of these energy shifts in terms of the number of circular polarised control polaritons,  $n_+$  and  $n_-$ , is given in Eqns. (S2).

$$\omega_{BS} = 2 |X_{11}|^2 |X_{12}|^2 \frac{(g_1 + g_2)}{2A_{\text{eff}}} (n_+ + n_-), \quad (\text{S2a})$$

$$\omega_Z = 2 |X_{11}|^2 |X_{12}|^2 \frac{(g_1 - g_2)}{A_{\text{eff}}} (n_+ - n_-), \quad (\text{S2b})$$

$$\frac{1}{A_{\text{eff}}} = \frac{\iint_{-\infty}^{\infty} I_{11} I_{12} \cdot dx dy}{\iint_{-\infty}^{\infty} I_{11} \cdot dx dy \cdot \iint_{-\infty}^{\infty} I_{12} \cdot dx dy}. \quad (\text{S2c})$$

Here  $|X_{11}|^2$  and  $|X_{12}|^2$  are the fractions of exciton in the makeup of the control and signal polaritons (the square moduli of the relevant Hopfield coefficients).  $A_{\text{eff}}$  is the effective nonlinear area which is an average over the transverse spatial distribution of the frequency blueshift (which has the spatial distribution of the control state) weighted by the intensity of the mode being perturbed (which has the spatial distribution of the signal state).  $I_{11}$  and  $I_{12}$  are the intensities of the  $E_{11}$  and  $E_{12}$  modes as a function of  $x$  and  $y$ . Note also the leading factor of 2 in the energy shifts which arises because cross-modulations between modes of different frequency and wavenumber are twice as strong as self-modulations<sup>1</sup>. We ignore the nonlinear contribution of the signal beam since the linearly polarised signal polaritons do not change  $\omega_Z$  and only add a diagonal matrix to the Hamiltonian that is

present whether the control beam is on or off. Thus any signal-beam nonlinear term just acts like an additional detuning.

Equations (S1) can be solved using matrix diagonalisation and integrating factors to give the field in Eqn. (S3).

$$u_x = \frac{P_x (\omega_{BS} - \Delta_p - i\gamma/2 - \omega_s/2) + iP_y \omega_Z/2}{(\omega_1 - \Delta_p)(\omega_2 - \Delta_p)} \quad (\text{S3a})$$

$$u_y = \frac{P_y (\omega_{BS} - \Delta_p - i\gamma/2 + \omega_s/2) - iP_x \omega_Z/2}{(\omega_1 - \Delta_p)(\omega_2 - \Delta_p)} \quad (\text{S3b})$$

$$\omega_1 = \omega_{BS} - i\gamma/2 + \omega_s \cos(\theta)/2 \quad (\text{S3c})$$

$$\omega_2 = \omega_{BS} - i\gamma/2 - \omega_s \cos(\theta)/2 \quad (\text{S3d})$$

$$\tan(\theta) = \omega_Z/\omega_s \quad (\text{S3e})$$

Here  $\omega_1$  and  $\omega_2$  are the eigenvalues of the Hamiltonian  $\mathcal{H}$ , which are the frequencies of the two polarisation split modes.  $\theta$  is an angle characterising the relative strength of the interaction-induced circular polarisation splitting and the intrinsic pillar linear polarisation splitting. It can be seen that in general the nonlinearity changes the output polarisation in two ways. It changes the frequencies of the two states relative to the signal laser and it changes the eigenvectors of  $\mathcal{H}$  from linear polarisation states to slightly elliptical, thus changing their relative overlaps with the signal laser.

The light escaping from the pillar toward the detection apparatus has the same coherence and polarisation as the internal micropillar polariton field. Thus the vector  $(u_x, u_y)^T$  is also a Jones vector describing the transmitted light. Writing the vector as  $(|u_x| \exp(i\phi_x), |u_y| \exp(i\phi_y))^T$  we can obtain the Stokes parameters given in Eqn. (S4), where we have  $S_0 = 1$  since we deal with fully coherent light derived from a laser.

$$S_1 = \frac{\rho - 1}{\rho + 1} \quad (\text{S4a})$$

$$S_2 = \frac{2\sqrt{\rho} \cos(\phi_x - \phi_y)}{\rho + 1} \quad (\text{S4b})$$

$$S_3 = \frac{-2\sqrt{\rho} \sin(\phi_x - \phi_y)}{\rho + 1} \quad (\text{S4c})$$

$$\rho = |u_x|^2 / |u_y|^2 \quad (\text{S4d})$$

Now that we have a Jones vector describing the output polarisation state from the pillar we can use standard Jones calculus to obtain the intensities at the two APDs. Since the signal beam is polarised along the  $y$  direction, parallel to the momentum of the  $E_{12}$  mode we can write  $P_x = 0$ . We set the detection half wave plate in the apparatus to balance the APDs e.g. for our vertically polarised laser the APDs are measuring the diagonal and anti-diagonal components. Thus we are measuring  $S_2$  given by

$$S_2 = \frac{|u_D|^2 - |u_A|^2}{|u_D|^2 + |u_A|^2}. \quad (\text{S5})$$

Inserting the solution Eqn. (S3) into Eqn. (S4) we now have an expression for the experimentally measured polarisation degree in terms of the state of the polariton system.

$$S_{\text{expt}} = \frac{2(\omega_Z/2)(\gamma/2)}{(\omega_{BS} - \Delta_p + \omega_s/2)^2 + (\gamma/2)^2 + (\omega_Z/2)^2} \quad (\text{S6})$$

If the field is expressed in a basis of circular polarised components some algebra reveals that the relative phase  $\phi$  between amplitudes of the right and left polarised components is given by  $\tan(\phi) = -S_2/S_1$ . Using Eqn. (S4) we obtain

$$\tan(\phi) = \frac{2(\omega_Z/2)(\gamma/2)}{(\omega_{BS} - \Delta_p + \omega_s/2)^2 + (\gamma/2)^2 - (\omega_Z/2)^2}. \quad (\text{S7})$$

Writing the numbers of controls polaritons as  $n_+ = n(1 + \cos 2\theta_c)/2$  and  $n_- = n(1 - \cos 2\theta_c)/2$  for  $(0 \leq \theta_c \leq \pi/2)$ , expanding Eqns. (S6) and (S7) to first order in the total number of control polaritons  $n$ , and making a small angle approximation for  $\phi$  we obtain

$$\Delta\phi \approx S_{\text{expt}} \approx S_{\text{max}} f(\Delta_p, \theta_c) \quad (\text{S8a})$$

$$S_{\text{max}} = \frac{2|X_{11}|^2 |X_{12}|^2 (g_1 - g_2) n}{A_{\text{eff}} (\gamma/2)} \quad (\text{S8b})$$

$$f(\Delta_p, \theta_c) = \frac{(\gamma/2)^2}{\Delta_{\text{eff}}^2 + (\gamma/2)^2} \cos 2\theta_c \quad (\text{S8c})$$

$$\Delta_{\text{eff}} = \Delta_p - \omega_s/2. \quad (\text{S8d})$$

We finally obtain that the nonlinear phase  $\Delta\phi$  accumulated between circular components is a Lorentzian function of signal laser detuning from resonance and has maximum value  $S_{\text{max}}$ . This maximum value is the value quoted for the expected phase shift in the main manuscript. It is proportional to the blueshift of one circularly polarised component of the signal state due to the circularly polarised control beam e.g. to the effective nonlinear Zeeman splitting induced by the control. The phase shift leads to a Faraday-like rotation of the linear polarisation angle, which is detected through the change in diagonal-antidiagonal polarisation degree  $S_2$ .

Physically,  $\theta_c$  represents the angle of a quarter wave plate used to set the control beam polarisation. In Fig. 2 in the main text we measure the case with  $\theta_c = 0$  so that  $n_+ = n$  and  $n_0 = 0$ , e.g. a fully circularly polarised control beam. As the control beam is switched to linear polarisation ( $\theta_c = \pi/4$ ) the expected phase shift and polarisation rotation vanish. When the control beam reaches the opposite circular polarisation ( $\theta_c = \pi/2$ ) the phase shift will have opposite sign to that at  $\theta_c = 0$ . This is shown experimentally in Fig. 3 in the main text.

While Eqn. (S8) is a first order approximation we can also calculate the nonlinear phase and change in polarisation degree exactly by using Eqns. (S3) and (S4). Supplementary Figure 3 shows the change in polarisation degree (solid coloured curves) and phase (dotted black

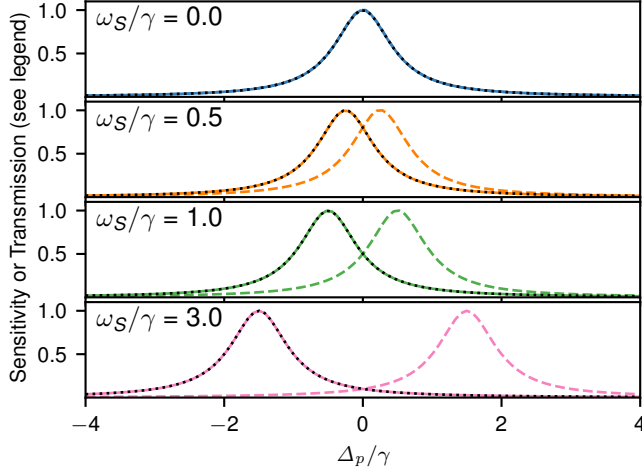

**Supplementary Figure 3. Exact nonlinear phase and change in polarisation degree.** Solid coloured curves show sensitivity  $[S_{\text{expt}}(n=1) - S_{\text{expt}}(n=0)]/S_{\text{max}}$ . Dotted black curves show nonlinear phase  $[\phi(n=1) - \phi(n=0)]/S_{\text{max}}$ . Dashed colored curves show total transmitted power  $|u_x|^2 + |u_y|^2$  normalised to the peak. The four panels show the results for four different linear polarisation splittings  $\omega_S$ . The parameters used in this calculation closely match the experimental ones and are  $\theta_c = 0$ ,  $P_y = 1$ ,  $P_x = 0$ ,  $g_2 = -0.1g_1$ ,  $\gamma = 83 \text{ } \mu\text{eV}$ ,  $\omega_Z(n=1)/(\gamma/2) = 3.7 \times 10^{-3}$ .

curves) between the cases with  $n = 1$  and  $n = 0$ . We consider four different TE-TM splittings  $\omega_S$ . The polarisation degree and phase agree with each other and have a peak at  $S_{\text{max}}$  exactly as predicted by the approximation. We will henceforth refer to the change in polarisation degree divided by  $S_{\text{max}}$  as the sensitivity. The figure also shows the power transmission (normalised to the peak) of the system as dashed lines. For zero TE-TM splitting the sensitivity and transmission lie on top of each other so that a maximum transmission implies maximum sensitivity. As the TE-TM splitting increases from one panel to another we see that the sensitivity peak and the transmission peak move in opposite directions. At large TE-TM splitting compared to the linewidth the sensitivity at peak transmission is very small. In our experiment the TE-TM splitting was smaller than the linewidth, as can be seen from the spectrum in Fig. 1b in the main text, and we tuned the laser frequency to maximise transmission. Thus we should observe a phase rotation close to  $S_{\text{max}}$ . Nevertheless, changes in laser detuning on the order of the linewidth can lead to a reduction in the observed nonlinear phase shift.

In the experiment small errors in setting the half-waveplate in the detection path sometimes occurred and only became apparent after collecting enough data to have good statistics. Using our model we have checked the effect of such deviations and found that they do not strongly affect results. For example, even if the diagonal or anti-diagonal component had twice the intensity of the other our measurement of polarisation degree would

underestimate the actual phase by only  $\sim 5\%$ .

### Supplementary Discussion 3. Data analysis

In this section we will give further details of the process by which we convert the raw photon counting traces into signal beam polarisation degrees with the control beam on and off, from which we obtain the nonlinear phase shift. As described in the main text, intensities are measured by avalanche photodiodes (APDs) connected to a time-correlated-single-photon-counting (TCSPC) card (Becker and Hickl SPC-630 with HRT-82 router)<sup>2</sup>. Single photon events from the APDs are sorted into time bins depending on their delay relative to a repetitive synchronisation signal to build up a histogram of arrival times. They are also sorted into one of four curves depending on which of the two APDs caused the event (each APD measures one polarisation component) and whether the control beam was on or off.

An example of the 4 curves is shown in Fig. 1f in the main text. The TCSPC system was synchronised to the pulses coming from the mode-locked Ti:Sapphire laser producing the  $\sim 100 \text{ ps}$  signal pulses. The laser repetition rate was 80 MHz, synchronisation was performed by directing a portion of the signal laser pulses onto a fast photodiode, and the TCSPC card operated in reverse start-stop configuration<sup>2</sup>. Since the synchronisation is derived from the signal pulses, the signal photons always appear in a fixed range of time bins in the TCSPC curves. This leads to the peaks seen in Fig. 1f in the main text. By contrast, photons arising from any processes which are not correlated with the 80 MHz repetition of the signal laser pulses are distributed equally across all time bins and appear as a CW background.

#### A. Background removal

Contributions to the CW background include APD dark and after-pulsing counts<sup>2</sup>, leakage of laboratory lighting through the detection optical path (although we measured with the main room lights off to minimise this effect) and scattered control beam light which is not completely excluded by the spectrometer owing to its diffuse nature. Most of the background is eliminated by taking a mean background level using points well separated from the peaks in the TCSPC trace and subtracting this background level from the curves. The CW background count rate is typically a few  $\times 10^4$  compared to  $\sim 10^6$  for the signal. Additionally we only select a window of 2-3 ns width in the TCSPC traces over which to integrate signal counts, whereas the background counts are spread over the whole 12.5 ns period of the synchronisation signal.

To check that the background does not affect the final results we extracted the nonlinear phase both with and without background subtraction and checked the difference. Supplementary Fig. 4 shows the extracted phase as

a function of the width of the integration window around the peak of signal pulses. The solid curves show the actual extracted phase while the dashed curves show the phase which would have been extracted without background subtraction. The vertical dotted lines give the window width used for the final values given in the paper. For small window widths the accumulated counts are low, resulting in larger uncertainty in the extracted phase. A larger window width accumulates more of the CW background counts. Without background subtraction this increasing background contribution leads the dashed curves to increase. By contrast, the solid curves are relatively independent of the window width which shows the background has been reduced to a negligible amount. The data we show here is for the higher control beam powers and the effect of the background is lower for lower powers.

### B. Signal counting statistics

Overall we collected  $N_{\text{photon}} = (1 - 3) \times 10^9$  signal photons (sum of all four channels), depending on the collection time. We collected photons for longer at the lower control powers to obtain better statistics. We found that there was good agreement between the measured error bar sizes  $2\sigma$  for the phase and those expected for the Poissonian counting statistics of the signal laser beam  $\sigma = 2/\sqrt{N_{\text{photon}}}$ . Here  $\sigma$  is the standard deviation in the phase shift  $\phi$ . This indicates that the main source of uncertainty within each data point is the counting statistics.

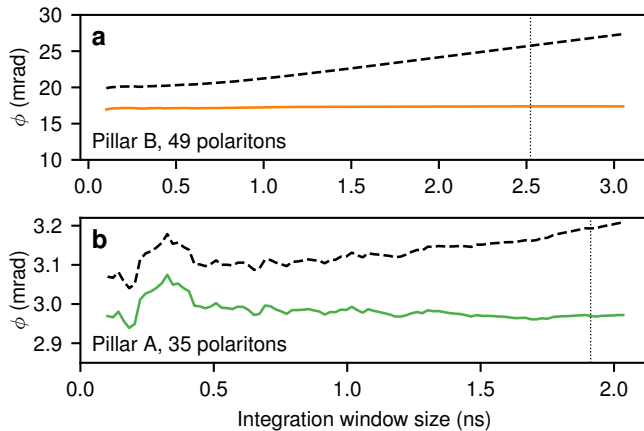

**Supplementary Figure 4.** Effect of integration window size on the extracted value of phase with (solid curves) and without (dashed curves) background subtraction. Vertical dotted lines give the window width used for the points in the main text.

### C. Counting rate and system dead times

The APDs were typically operated at a photon detection rate of less than  $2 \times 10^6$  counts per second each, equivalent to a combined 0.05 photons per period of the 80 MHz synchronisation signal. There is therefore only a very small probability of multiple photons arriving within one detection cycle. After a photon triggers an APD that APD is blind for the dead time  $t_d = 77$  ns. If a second photon arrives during this dead time it is lost. The higher the rate of arrival of photons at the APD the higher the counting loss. The counting loss effect is well understood<sup>2</sup> and the count rate which would occur in the absence of dead time photon loss,  $R_{\text{act}}$ , can be obtained from the measured count rate  $R_{\text{meas}}$  using the formula  $R_{\text{act}} = R_{\text{meas}} / (1 - t_d R_{\text{meas}})$ . With our photon detection rate we operate several times below the maximum useful counting rate of  $1/2t_d = 6.5 \times 10^6$  and only lose about 15% of the photons through counting loss. To ensure that this did not affect the results we applied the counting loss correction formula to the measured intensities. We found that the phase shifts always increased, typically by an amount of order 10%. In the data presented in the paper we do not apply this dead time correction in order to avoid over-analysing the data. As well as the APD dead time there is also a dead time in the TCSPC card while detected photons are processed by the electronics. However, since the signal from both APDs are combined by the router before being sent to the TCSPC card this dead time affects both APD channels equally. Since we calculate a polarisation degree, this overall attenuation of both polarisation components cancels out.

### Supplementary Discussion 4. Experimental measurement of transmitted power

The power transmitted through the sample was measured using the integrated counts accumulated on a CCD camera. We calibrated the CCD by transmitting a laser through the etched portion of the sample, which consists of the GaAs substrate and an anti-reflection coating. Using a high laser power  $\sim 100 \mu\text{W}$  and a commercial power meter we confirmed that the transmitted power was 68%, matching the expected Fresnel power transmission through the air/GaAs interface. The laser was then attenuated by a known fraction using commercial neutral density filters, which were pre-calibrated using the laser at the same wavelength and a commercial power meter. The attenuated laser was sent to the CCD camera and the intensity recorded. The laser was then optimally coupled to the micropillar cavity and the intensity of the micropillar transmission recorded. This allowed the pillar transmission to be compared to the known substrate transmission. The laser travels along exactly the same path to the CCD when transmitted through either the substrate or the pillar. With the well-calibrated transmission we then obtain the transmitted power from the

incident power, and finally the number of polaritons in the cavity, following the argument in supplementary discussion 5.

### Supplementary Discussion 5. Determining number of polaritons from transmitted power

In this section we will show that for a cavity with parameters in a range consistent with our experimental measurements the energy (number of particles) in the cavity can be deduced from the transmitted power with high accuracy from a simple formula (Eqn. (S11)). We initially consider the case of a cavity without losses and derive Eqn. (S11) with a very simple argument. We will then present an exact numerical solution of Maxwell's equations including losses and materials dispersion and show that Eqn. (S11) is a highly accurate approximation for a simulated cavity with parameters in a wide range around those measured for our cavity.

#### A. Simplified model

We initially consider energy  $E_{\text{cav}}$  circulating in a cavity containing a lossless medium between two partially transparent mirrors as described in Ref. 3. We will denote the top mirror, where the pump beam is incident, as DBR1 and the bottom mirror, through which the light is transmitted towards the detectors, as DBR2. The cavity is pumped continuously by a monochromatic light source so that it reaches a steady state and contains a constant amount of energy. On each round trip of the energy in the cavity the mirrors reflect fractions  $R_{\text{DBR1}}$  and  $R_{\text{DBR2}}$  back into the cavity while a fraction  $T_{\text{DBR2}}$  is transmitted through DBR2 to be detected. A fraction  $T_{\text{DBR1}}$  is also transmitted in the reverse direction and interferes (typically destructively) with the direct reflection of the pump beam from mirror 1 to produce the overall reflection. The steady state condition is such that the energy  $E_{\text{cav}}$  and round-trip transmitted fraction  $T_{\text{DBR2}}$  lead to the expected overall cavity power transmission<sup>3</sup>.

With energy  $E_{\text{cav}}T_{\text{DBR2}}$  transmitted on each round trip, the time-averaged transmitted power is then  $P_{\text{out}} = E_{\text{cav}}T_{\text{DBR2}}/t_{\text{rt}}$  where  $t_{\text{rt}}$  is the round trip time. Meanwhile, the finite cavity linewidth arises from the losses through both mirrors and can be written as  $\gamma_{\text{DBR}} = -\ln(R_{\text{DBR1}}R_{\text{DBR2}})/t_{\text{rt}} \sim (T_{\text{DBR1}} + T_{\text{DBR2}})/t_{\text{rt}}$ . Eliminating  $t_{\text{rt}}$  from these expression results in Eqn. (S9).

$$E_{\text{cav}} = \hbar\omega N_{\text{pol}} = \frac{P_{\text{out}}}{\eta \cdot \gamma_{\text{DBR}}} \quad (\text{S9a})$$

$$\eta = \frac{-T_{\text{DBR2}}}{\ln(R_{\text{DBR1}}R_{\text{DBR2}})} \sim \frac{T_{\text{DBR2}}}{T_{\text{DBR1}} + T_{\text{DBR2}}} \quad (\text{S9b})$$

Here  $N_{\text{pol}}$  is the number of photons in the cavity and  $\eta$  is a mirror asymmetry factor which characterises the transmission through the mirror on the detection side com-

pared to the total cavity losses due to non-unity reflection of the mirrors. Furthermore,  $\gamma_{\text{DBR}}$  is the linewidth (FWHM) of the cavity in the absence of loss and in the photon-only limit (no coupling to excitons) so that it characterises the rate of outcoupling through the mirrors alone.

If we now imagine adding an exciton resonance so that the system enters the strong photon-exciton coupling regime then we must account for the fact that only a fraction  $|C|^2$  of the cavity energy circulates as photons in order to be coupled out. Assuming for the moment that the excitonic losses and nonlinearity are negligible, the main effect of adding the exciton resonance is to reduce the average energy transport velocity in the cavity by a factor of the photon fraction  $|C|^2$  causing an increase in round trip time and hence a reduction in both the cavity linewidth and the output power for a given cavity energy. The energy and transmitted power will then be related by Eqn. (S10) where  $\gamma_{\text{d}} = \gamma_{\text{DBR}}|C|^2$  and  $\gamma_{\text{DBR}}$  is the cavity linewidth without strong coupling. We note that this effect occurs for any change in the dispersive properties of the cavity, not just strong coupling, though in those cases  $\gamma_{\text{d}}$  will take a different form.

$$E_{\text{cav}} = \frac{P_{\text{out}}}{\eta\gamma_{\text{d}}} \quad (\text{S10})$$

In principle Eqn. (S10) could be used with the measured polariton linewidth  $\gamma$  at the frequency of interest substituted in for  $\gamma_{\text{d}}$ . However, additional contributions to the linewidth due to exciton dephasing<sup>4</sup> make this problematic. It is not possible in the experiment to partition the polariton linewidth into the contributions from tunneling through the mirrors (transmission) and from exciton-related effects. For this reason it is more accurate to work with an experimentally determined value  $\gamma_{\text{DBR}}$  and scale by the photon fraction. A caveat here is that in a real experiment, where the quantum well cannot be added and removed,  $\gamma_{\text{DBR}}$  will usually have to be measured at a frequency lower than the one of interest, where the exciton contribution is negligible. If the refractive indexes  $n$  and dispersion  $\partial n/\partial\omega$  of the underlying cavity materials (AlGaAs in our case) change significantly between the operating frequency and that at which  $\gamma_{\text{DBR}}$  is measured then it can introduce a systematic error. Fortunately, the GaAs refractive index varies much more slowly with frequency than the quantum well resonance so the difference is small over the detunings which must be used in practice. The relation Eqn. (S11) may then be used to obtain the cavity energy from the transmitted power in the strongly coupled case. Here  $\gamma_{\text{T}} = \eta \cdot \gamma_{\text{DBR}}$  may be interpreted as the fraction of the total cavity radiative linewidth associated with transmission through DBR2 towards the detector.

$$E_{\text{cav}} = \hbar\omega N_{\text{pol}} = \frac{P_{\text{out}}}{\gamma_{\text{T}}|C|^2} \quad (\text{S11})$$

For accurate results  $\gamma_{\text{DBR}}$  should be obtained experi-

mentally and not through simulation alone. This is because it is sensitive to differences in the material compositions and layer thicknesses between the nominal values and the ones in the actual sample. We measured  $\gamma_{\text{DBR}}$  at large negative detuning on the planar microcavity before it was etched into pillars. We measured a value  $\gamma_{\text{DBR}} = 20 - 30 \mu\text{eV}$ . Values from transfer matrix simulations of the cavity (see below) are in good agreement, giving values of  $18.9 \mu\text{eV}$  or  $30.7 \mu\text{eV}$  depending on the values used for the AlGaAs refractive indexes (respectively, the model values from Ref. 5, or the experimental values from Ref. 6 shifted in energy by the bandgap shift of GaAs to account for the different temperature). We take  $\gamma_{\text{DBR}} = 25 \pm 5 \mu\text{eV}$  as the value used in the main text. As we confirm later, the parameter  $\eta$  can safely be obtained from the simulations since it depends only on the *ratio* of mirror transmissions, which is only weakly sensitive to the refractive indexes and is determined largely by the number of repeats in the DBRs. The experimental accessibility of the important parameters is the reason for using Eqn. (S9). We now go on to show that it provides an accurate approximation to the actual ratio of transmitted power and cavity energy determined from solution of Maxwell's equations.

## B. Exact electromagnetic model

We use a transfer matrix<sup>7</sup> approach to exactly solve Maxwell's equations for a planar cavity structure. We consider a planar structure since exact results are easily available and the energy storage and power transmission are determined by the layered mirror/cavity structure in the longitudinal direction. In the etched micropillar system there is also the question of mode-matching of the incident laser beam to the transverse mode profiles of the square pillar structure. However, poor mode matching only changes the excitation efficiency in the same way as a frequency detuning of the excitation laser away from resonance. As we will show below, such detunings from resonance do not change the ratio of the output power to the energy in the cavity. Since we experimentally measure the power coming out from the cavity the mode-matching at the input does not matter.

We consider a planar multilayer structure with interfaces perpendicular to the  $z$  direction and surrounded on either side by semi-infinite media as depicted in Fig. 5. The material permittivities are isotropic, homogeneous within each layer and frequency dependent. The materials are non-magnetic and passive (no gain) but may be lossy so that they can have complex permittivity with a positive imaginary part. Since the structure is planar and has translational symmetry in the  $x$  and  $y$  direction the electromagnetic normal modes are plane waves with electric field  $[\mathbf{E}(z) \exp(i\mathbf{k}_{\parallel} \cdot \mathbf{r}_{\parallel} - i\omega t) + \text{c.c.}] / 2$ , and similar for the magnetic field, where c.c. denotes the complex conjugate of the preceding term. Here  $\mathbf{k}_{\parallel} = k_x \hat{\mathbf{x}} + k_y \hat{\mathbf{y}}$ ,  $\mathbf{r}_{\parallel} = \mathbf{x} + \mathbf{y}$  where the in-plane wavenumber components

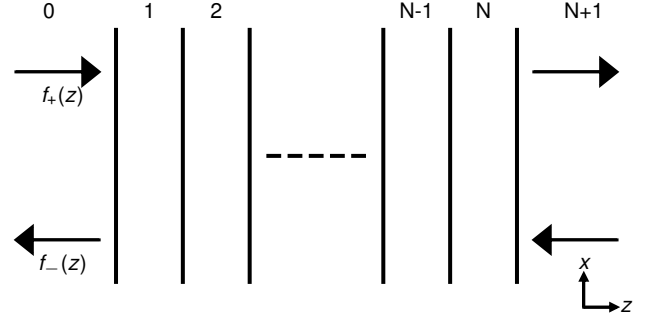

**Supplementary Figure 5.** Schematic of a layer structure and the notation used for transfer matrix calculations.

$k_x$  and  $k_y$  are the same in every layer.  $\hat{\mathbf{x}}$  and  $\hat{\mathbf{y}}$  are unit vectors in the  $x$  and  $y$  directions. The  $z$  component of wavenumber is given by  $k_z(z) = \sqrt{(k_0 n(z))^2 - k_{\parallel}^2}$  where  $k_0 = \omega/c_0$ ,  $c_0$  is the speed of light in vacuum, and  $k_{\parallel} = |\mathbf{k}_{\parallel}| = \sqrt{\mathbf{k}_{\parallel} \cdot \mathbf{k}_{\parallel}^*}$  is the magnitude of  $\mathbf{k}_{\parallel}$ . The refractive index  $n(z)$  is different in each layer and so is a piecewise function of  $z$ . Thus  $k_z(z)$  is also a piecewise function of  $z$ . In general there is a forward and a backward propagating wave in each layer. In what follows we designate the symbol  $k_z$  as the solution of the square root with positive real and imaginary part, which is the wavevector component of the forward propagating wave. The backward propagating wave then has momentum  $z$ -component equal to  $-k_z$ .

Since the structure is planar and the material properties are piecewise continuous Maxwell's equations can be solved in each layer as if it were a continuous medium and the solutions matched between layers using boundary conditions (also derived from Maxwell's equations). The translational symmetry also means that the solutions can be fully described by two decoupled polarisations denoted TE and TM. We introduce the per-polarisation scalar complex amplitudes  $f_+(z)$  and  $f_-(z)$  describing the forward and backward propagating waves. Without loss of generality we define the coordinate system so that the plane waves have wavevector in the  $x$ - $z$  plane. For the TE polarisation the electric and magnetic field components are then given by Eqns S12.

$$E_y(z) = f_+(z) + f_-(z) \quad (\text{S12a})$$

$$H_z(z) = [f_+(z) + f_-(z)] \sin \theta(z) / \eta(z) \quad (\text{S12b})$$

$$H_x(z) = -[f_+(z) - f_-(z)] \cos \theta(z) / \eta(z) \quad (\text{S12c})$$

$$H_y = E_x = E_z = 0 \quad (\text{S12d})$$

For the TM polarisation the field components are given by Eqns S13.

$$H_y(z) = [f_+(z) + f_-(z)] / \eta(z) \quad (\text{S13a})$$

$$E_z(z) = -[f_+(z) + f_-(z)] \sin \theta(z) \quad (\text{S13b})$$

$$E_x(z) = [f_+(z) - f_-(z)] \cos \theta(z) \quad (\text{S13c})$$

$$E_y = H_x = H_z = 0 \quad (\text{S13d})$$

Here,  $\sin \theta = k_{||} / (k_0 n(z))$ ,  $\cos \theta = k_z(z) / (k_0 n(z))$ , and the impedance  $\eta = \eta_0 \eta_r(z)$  where  $\eta_0$  is the impedance of free space and the relative impedance  $\eta_r(z) = 1/n(z)$  (remembering that we work with non-magnetic materials so that the relative magnetic permeability is unity). These are all piecewise continuous functions of  $z$ . Writing the functions  $f_+(z)$  and  $f_-(z)$  as a two-component vector, their values within a layer can be calculated using Eqn. (S14) in compact matrix notation.

$$\begin{pmatrix} f_+(z) \\ f_-(z) \end{pmatrix} = \begin{pmatrix} e^{i\phi} & 0 \\ 0 & e^{-i\phi} \end{pmatrix} \begin{pmatrix} f_+(z_R) \\ f_-(z_R) \end{pmatrix} \quad (\text{S14a})$$

$$\phi = k_z(z - z_R) \quad (\text{S14b})$$

Here,  $z_R$  is the  $z$ -coordinate of the right hand edge of the layer and  $(f_+(z_R), f_-(z_R))^T$  are the amplitudes at the right hand edge of the layer. The amplitudes at the left hand edge of the layer are obtained simply by inserting  $z = z_L$  in Eqn. (S14) where  $z_L$  is the  $z$ -coordinate of the left hand edge.

The relation between the amplitudes in adjacent layers is given by Eqn. (S15), which are obtained from the Maxwell boundary conditions.

$$\begin{pmatrix} f_+^{(m)} \\ f_-^{(m)} \end{pmatrix} = \begin{pmatrix} \frac{\rho + \rho_z / \rho}{2} & \frac{\rho - \rho_z / \rho}{2} \\ \frac{\rho - \rho_z / \rho}{2} & \frac{\rho + \rho_z / \rho}{2} \end{pmatrix} \begin{pmatrix} f_+^{(m+1)} \\ f_-^{(m+1)} \end{pmatrix} \quad (\text{S15a})$$

$$\rho_z = k_z^{(m+1)} / k_z^{(m)} \quad (\text{S15b})$$

$$\rho^{\text{TM}} = n^{(m+1)} / n^{(m)} \quad (\text{S15c})$$

$$\rho^{\text{TE}} = 1 \quad (\text{S15d})$$

Here,  $(f_+^{(m)}, f_-^{(m)})^T$  are the amplitudes at the right hand edge of layer  $m$  and  $(f_+^{(m+1)}, f_-^{(m+1)})^T$  are the amplitudes at the left hand edge of layer  $m+1$ .  $k_z^{(m)}$  and  $n^{(m)}$  are the values of  $k_z$  and  $n$  in layer  $m$ , and similar for layer  $m+1$ . The value of  $\rho$  is different for TE and TM polarisations and is given by  $\rho^{\text{TE}}$  and  $\rho^{\text{TM}}$  respectively.

The simulations were performed in the following way. For a given frequency  $\omega$  we calculated the refractive indexes of the materials at that frequency. We initialised the amplitudes on the left hand side of layer  $N+1$  (the right hand semi-infinite medium) to  $(1, 0)^T$ . We then applied Eqns. (S14) and (S15) repeatedly to calculate  $(f_+(z), f_-(z))^T$  for all positions  $z$ , finishing in the left hand semi-infinite medium, layer 0.

Having obtained the fields as a function of  $z$  we may then obtain the time-averaged Poynting vector given in Eqn. (S16).

$$\mathbf{S}(z) = \text{Re}[\mathbf{E}(z) \times \mathbf{H}^*(z)] / 2 \quad (\text{S16})$$

Here the symbol  $\text{Re}$  denotes taking the real part. This gives the net energy flux density at any given point in the structure. The output power from the structure can then be written  $P_{\text{out}} = |S|$  for  $S$  in the right hand semi-infinite medium. Using the Poynting vector in layer 0 with  $f_-$  set to zero we obtain the incident intensity and divided the amplitudes  $(f_+(z), f_-(z))^T$  through by its square root so that the calculated fields are always those for unit incident intensity. The Poynting vector in layer  $N+1$  then gives the transmission of the structure.

For quasi-monochromatic fields occupying a narrow frequency range, as we use in this experiment, the electric and magnetic energy densities may be written as in Eqn. (S17) with the total stored electromagnetic energy density being  $W(z) = W_E(z) + W_H(z)$ .

$$W_E(z) = \frac{1}{4} \epsilon_0 \epsilon_{\text{e.d.}} |\mathbf{E}(z)|^2 \quad (\text{S17a})$$

$$W_H(z) = \frac{1}{4} \mu_0 |\mathbf{H}(z)|^2 \quad (\text{S17b})$$

$$\epsilon_{\text{e.d.}} = 1 + \left| \frac{\partial [\omega (\epsilon_r - 1)]}{\partial \omega} \right| \quad (\text{S17c})$$

Here,  $\epsilon_0$  and  $\mu_0$  are the permittivity and permeability of free space respectively and  $\epsilon_r$  is the (possibly complex) relative permittivity. The factor  $\epsilon_{\text{e.d.}}$  accounts for the contribution of dispersion and loss to the electric energy density. We have used the form from Ref. 8 which, in the limit of zero loss, reduces to the well known expression for dispersive non-lossy materials<sup>9</sup>  $\partial [\omega \text{Re}(\epsilon)] / \partial \omega$  while also reproducing the analytical results due to Loudon<sup>10,11</sup> for Lorentzian oscillators with strong loss and dispersion. The latter are often used to represent the excitonic optical resonance in simulations of polariton systems. The total energy stored in the cavity can then be determined by integrating the energy density in the multilayer. We do not include any energy in the semi-infinite regions outside the multilayer since this can never be reflected back inside the cavity in order to contribute to the nonlinear response.

### C. Solutions of the electromagnetic model

We now go on to present calculated values of the linewidth, transmitted power and energy stored in the cavity for a range of parameters around those of the actual cavity used in the experiments. For these calculations the refractive indexes were obtained from the model given in Ref. 5. The linewidths of the cavity structure were obtained by calculating the transmission for a range

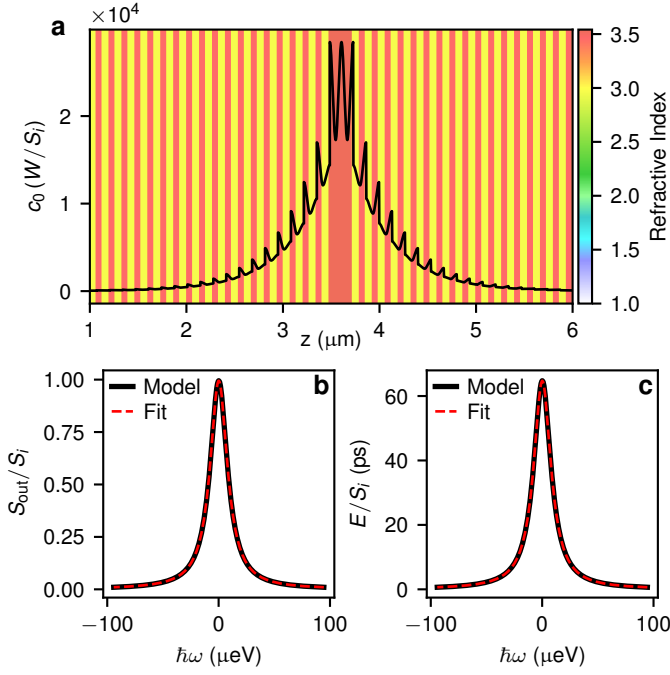

**Supplementary Figure 6.** Power transmission through and energy density in a DBR cavity. (a) Electromagnetic energy density per unit incident intensity as a function of distance into the structure from the first interface on the incident side. Colour scale indicates the real part of the material refractive index. The in-plane incidence angle is zero and the frequency of the wave is exactly on resonance with the cavity mode.  $c_0$  is the speed of light in free space. (b) Calculated power transmission (solid black) and Lorentzian fit (dashed red) as a function of the frequency of the incident wave. (c) Calculated total energy in the multilayer (solid black) and Lorentzian fit (dashed red) as a function of the frequency of the incident wave.

of wavelengths about resonance and fitting a Lorentzian to the resulting peak. In this way variation of the material refractive indexes with wavelength is automatically taken into account. When calculating the energy density through Eqn. (S17) the wavelength dependence of refractive indices was included explicitly by numerically differentiating the refractive indices.

Supplementary Figure 6(a) shows the calculated energy density  $W$  (energy per unit volume) per unit incident intensity  $S_i$  (power per unit area) as it varies through the structure for the exactly resonant case. In the units of the figure the incident wave in free space has  $c_0W/S_i = 1$  where  $c_0$  is the speed of light in free space. Thus it can be seen that the energy density in the cavity is strongly enhanced (on the order of  $10^4$  times) over that in free space. The energy density consists of a piecewise factor resulting from the different material permittivities multiplied by an exponentially decaying envelope. When we integrate  $W$  over  $z$  to obtain the total energy  $E$  the contributions from spatial regions away from the center of the cavity are negligible. Supplementary Figure 6(b) shows the transmission (transmitted power  $S_{\text{out}}$

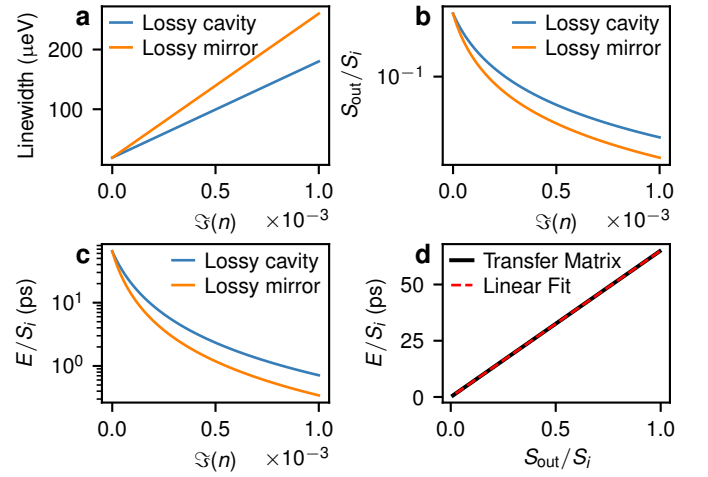

**Supplementary Figure 7. Effect of loss.** a Change of cavity mode linewidth with increasing imaginary part of the refractive index,  $\Im(n)$ , of either the cavity material (GaAs) or the high index mirror material ( $\text{Al}_{0.1}\text{Ga}_{0.9}\text{As}$ ). b Transmission through the cavity vs. loss. c Energy stored in the cavity vs. loss. d Energy stored in the cavity (from panel c) vs. transmission from panel b and best fit straight line.

divided by incident power  $S_i$ ) vs. the frequency of the incident wave. This is equivalent to an experiment where a very narrow single mode laser is tuned through the cavity resonance while the transmission is recorded. Since the cavity is close to being balanced the peak transmission is near unity. We note here that although the substrate mirror has more pairs the substrate is coated with an anti-reflection coating whereas the other mirror terminates with a GaAs/Air interface. The additional Fresnel reflection at this GaAs/Air interface mostly compensates the higher number of mirror pairs in the substrate mirror. The best fit Lorentzian function is plotted on top demonstrating that the lineshape is Lorentzian to a very high precision. Supplementary Figure 6(c) shows the total energy in the cavity divided by incident power. The Lorentzian fit has the same linewidth and central frequency as the output power to better than 2 parts in  $10^{-7}$ . This shows that the energy  $E$  and transmitted power  $S_{\text{out}}$  have a fixed ratio independent of frequency. We have also checked that the ratio of power and energy is constant for varying in-plane wavenumber at fixed frequency. Since the orthogonal transverse modes in a pillar structure are equivalent to the in-plane wavenumber modes of a planar structure we can be confident that non-optimal excitation of a micro-pillar does not affect the ratio of energy and transmitted power.

Supplementary Figure 7 shows the effect of material loss. We introduced loss by increasing the imaginary part of the refractive index in either the GaAs material of the cavity layer or of the  $\text{Al}_{0.1}\text{Ga}_{0.9}\text{As}$  material making up the high refractive index layers in the DBR mirror. The GaAs is the material where absorptive loss is most likely to arise in experiment as the light is very far from the

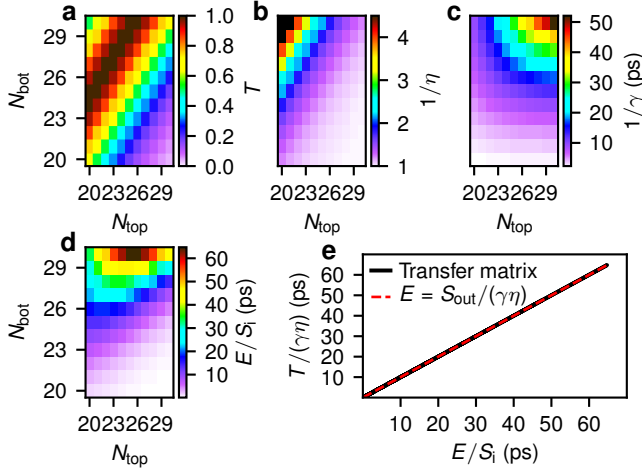

**Supplementary Figure 8. Effect of mirror reflectivities.** **a-d** show, respectively, peak transmission,  $1/\eta$ , inverse linewidth, and stored energy vs. number of DBR mirror pairs on the top and bottom of the structure. In the experimental structure  $N_{\text{top}} = 26$ ,  $N_{\text{bot}} = 30$ . **e** Transmitted power corrected for tunneling rate  $\gamma$  and cavity asymmetry  $\eta$  vs. stored energy. The solid black shows the values from the transfer matrix calculations for the various numbers of top and bottom mirror pairs while the dashed red curve is a straight line of gradient 1 passing through the origin.

band edge in the higher aluminium content layers. We simulated loss in the DBR only for completeness. Supplementary Figures 7a and b show that, as expected, the cavity mode linewidth increases and the transmitted power decreases with increasing loss. Supplementary Figure 7c shows that the energy stored in the cavity also decreases with increasing loss. Finally, Fig. 7d compares the stored energy and transmitted power from Fig. 7b and c respectively and shows that the two are directly proportional to each other. Thus we can conclude that absorptive loss reduces both the transmitted power and the energy in the cavity in proportion and so does not affect the ratio.

Supplementary Figure 8 shows the effect of changing the number of top and bottom DBR mirror pairs  $N_{\text{top}}$  and  $N_{\text{bot}}$ . In Fig. 8(a) it can be seen that the peak transmission, near to unity, is highest when the bottom mirror has approximately 4 more pairs than the top mirror. These points are where the top and bottom reflectivities are equal since the extra mirror pairs on the bottom side compensate the large Fresnel reflection at the GaAs/air interface on the top side (there is no strong Fresnel reflection on the bottom side due to the substrate anti-reflection coating). Fig. 8(b) illustrates the cavity asymmetry  $\eta$  (see Eqn. (S9b)). For equal top and bottom reflectivities half the cavity power is transmitted to the detection side so that  $1/\eta = 2$ , which coincides with the highest transmission points in Fig. 8(a). Fig. 8(c) shows that the cavity lifetime  $1/\gamma$  increases with increasing numbers of mirror pairs, as expected.

Fig. 8(d) shows the energy stored in the cavity which, in agreement with Eqn. (S11), is the product of the functions shown in Fig. 8(a-c). This is shown more explicitly in Fig. 8(e) where the two sides of Eqn. (S11) are plotted against each other (solid black line) using the values of  $T$ ,  $\gamma$ ,  $\eta$  and  $E$  obtained from the transfer matrix calculations for various  $N_{\text{top}}$  and  $N_{\text{bot}}$ . For comparison, the red dashed line is Eqn. (S11). From these it can be seen that the transfer matrix outputs satisfy Eqn. (S11) to a high degree of accuracy for a wide range of  $N_{\text{top}}$  and  $N_{\text{bot}}$ . Comparing the experimentally measured linewidth with the range in Fig. 8(c) confirms that our experimental device lies in this range where Eqn. (S11) works well.

We also varied the material compositions of the DBRs and found that changing the composition of the high aluminium content layer between  $\text{Al}_{0.93}\text{Ga}_{0.07}\text{As}$  and  $\text{Al}_{0.97}\text{Ga}_{0.03}\text{As}$  changed  $\eta$  between 0.542 and 0.530. Changing the low aluminium content layer between  $\text{Al}_{0.08}\text{Ga}_{0.92}\text{As}$  and  $\text{Al}_{0.12}\text{Ga}_{0.88}\text{As}$  changed  $\eta$  between 0.527 and 0.545. For the nominal material parameters of the experimental structure we obtain  $\eta = 0.536$ . Thus experimentally reasonable fluctuations in the MBE-grown materials lead to only a few percent change in  $\eta$ , confirming that  $\eta$  can safely be obtained from simulations.

In addition to the dependencies detailed above we also checked the effect of material dispersion, that is the frequency dependence of the refractive indices of the materials making up the structure. This is important to check since our cavity is composed of GaAs and we operate near the band edge where the dispersion is strong. The check was accomplished by setting the refractive index of all materials equal to a constant (wavelength-independent) value equal to the value at the resonant wavelength and comparing the results to the case where the refractive indexes vary with wavelength. We found that the material dispersion changes both the energy stored in the cavity and also the linewidth. Meanwhile the transmission at the peak is unaffected since it depends only on the refractive index values at the resonance frequency and not on their derivatives with frequency. The linewidth and stored energy are changed in proportion so that Eqn. (S11) still applies independent of the amount of material dispersion. Qualitatively, this occurs because the averaged velocity of energy transport relates the intra-cavity energy flux and energy density as well as determining the cavity round trip time and hence linewidth.

In conclusion we have shown using exact solution of Maxwell's equations that Eqn. (S11) can be used to determine the ratio of energy stored in the cavity to transmitted power. When experimentally determined values are used for the lossless cavity linewidth  $\gamma_{\text{DBR}}$  there is no need for detailed knowledge of the material refractive indexes or their dependence on wavelength as these do not affect the ratio.

### Supplementary Discussion 6. Phase shift estimates for a fiber cavity

In our device the phase shifts are limited by the linewidth  $\gamma=83 \text{ } \mu\text{eV}$ , exciton fractions  $|X_{11}|^2 \times |X_{12}|^2 = 0.105$ , and the large transverse area of the mode in the  $5 \text{ } \mu\text{m}$  square pillar. To estimate the possibility of achieving larger phase shifts in other setups we consider the system in Ref.<sup>12</sup>, where a high quality fiber microcavity was studied.

The authors measured the minimal second-order coherence function at zero delay, and observed antibunching of  $g_{\text{exp}}^{(2)}(0) = 0.95$ . From this they deduce the ratio of single polariton interaction energy to linewidth  $U_{\text{pp}}/\gamma = 0.088$ . Using this ratio we can now estimate the phase shifts which could be achieved in that system. We first account for some differences between the anti-bunching and XPM experimental approaches. We use interactions between co-circularly polarised polaritons rather than the linearly polarised polaritons used in Ref. 12. The relative interaction strengths are given by  $g_{\text{XX,circ}}/g_{\text{XX,lin}} = 2(g_1 - g_2)/(g_1 + g_2)$ . Using the common assumption that  $g_2 = -0.1g_1$ <sup>13</sup> we have  $g_{\text{XX,circ}}/g_{\text{XX,lin}} \sim 2.44$ . The effective area for interactions between control and signal pillar states is about 1.5 times larger than for interactions involving only the ground state. We may use an exciton fraction 0.6 and linewidth  $60 \text{ } \mu\text{eV}$  for the signal state since these are achievable in Ref. 12. The control state should be lower in energy by  $\sim 1 \text{ meV}$  to achieve spectral separation of the control and signal beams, as in this work. Thus we have ground state exciton fraction 0.34.

Taking all these into account  $[(2.44/1.5) \times (0.34/0.6) = 0.92]$  we may then expect the same polariton interaction energy as in Ref.<sup>12</sup>. We can then expect XPM phase shift  $2U_{\text{pp}}/(\gamma/2) = 320 \text{ mrad}$ , two orders of magnitude larger than measured in this paper. This arises due to the smaller modal area, higher exciton fractions and smaller linewidths in Ref. 12.

### Supplementary Discussion 7. Cascaded CPHASE gate with cross-Kerr nonlinearity

We observed phase shift due to cross-Kerr effect that corresponds to the conditional quantum operation. However, it was noted that a single cavity cross-Kerr interaction can not be seen as a controlled Pauli  $Z$  (CZ) quantum gate, as the interaction leads to mode entanglement in the frequency domain, and spoils the fidelity of the operation<sup>14–16</sup>. At the same time, it was shown that cascaded systems where nonlinearity is distributed between several cavities can overcome this problem<sup>17,18</sup>. In this section, we follow the cascaded scheme from Refs.<sup>18,19</sup> to show that controlled phase (CPHASE) gate based on exciton-polaritons may be arranged in a carefully engineered lattice system.

We start by recalling that our system can be seen as an effective two-mode cavity with the cross-Kerr interaction  $\chi$ , described by the effective Hamiltonian

$$H = H_1 + H_2 + H_{\text{int}} \equiv \Delta_a \hat{a}^\dagger \hat{a} + \Delta_b \hat{b}^\dagger \hat{b} + \chi \hat{a}^\dagger \hat{a} \hat{b}^\dagger \hat{b}, \quad (\text{S18})$$

where we use the rotating frame, introducing relative detunings  $\Delta_{a,b}$  for two polaritonic modes  $\hat{a}$  and  $\hat{b}$ . For simplicity the two can be considered equal,  $\Delta_{a,b} = \Delta$ , as non-zero detuning only introduces additional single particle phase shift, while not changing the two-particle quantum operation. We note that, when applied to the polaritonic system, the strength of cross-Kerr interaction  $\chi$  is related to polariton nonlinearity as  $\chi = 2U_{\text{pp}}$ .

To harness the effects of nonlinearity in the distributed fashion, we need to consider a lattice of polariton cavities (i.e. micropillars) that have edge states with suppressed backscattering<sup>20,21</sup>. This will be equivalent to having a circulator for each mode, being an essential tool for cascading. To describe the system, we use the *SLH* framework. It can be seen as a generalized input-output theory that conveniently describes various cascaded systems. Here,  $S$  corresponds to a scattering matrix (or matrices) of an element in the chain, that in our case is a nonlinear optical resonator. It is a unitary matrix that relates the input state  $|\nu\rangle$  to the output state  $|\omega\rangle$  as  $|\omega\rangle = S|\nu\rangle$ .  $L$  denotes the Lindblad-type dissipation term (jump operator) that describes the in/out coupling for the mode. Operator  $H$  is for the Hamiltonian that describes the unitary dynamics of the system. For more information we refer to review in Ref.<sup>22</sup>. Using *SLH* framework we can describe multi-cavity scattering, and define a CPHASE gate fidelity from single- and two-photon scattering matrices. First, a single-photon scattering matrix  $S_1$  can be derived from using input-output relations as

$$S_1(\omega_a; \nu_a) = -\frac{\Gamma^*(\omega_a)}{\Gamma(\omega_a)} \delta(\omega_a - \nu_a), \quad (\text{S19})$$

where  $\nu_a, \omega_a$  are input and output frequencies, and we defined an auxiliary function  $\Gamma(\omega) := \gamma/2 + i(\Delta - \omega)$ . Similar expression can be derived if photon propagates as a wavepacket with some envelope in the frequency domain  $\xi(\omega)$ . One can proceed to derive two-photon scattering matrix, getting

$$S_2(\omega_a, \omega_b; \nu_a, \nu_b) = S_1(\omega_a; \nu_a) S_1(\omega_b; \nu_b) - i \frac{\chi \gamma^2}{\pi} \left( 1 + \frac{2i\chi}{\Gamma(\omega_a) + \Gamma(\omega_b)} \right)^{-1} \frac{\delta(\omega_a + \omega_b - \nu_a - \nu_b)}{\Gamma(\omega_a) \Gamma(\omega_b) \Gamma(\nu_a) \Gamma(\nu_b)}, \quad (\text{S20})$$

where the first term corresponds to the single photon contributions, and the second term introduces the effect of cross-Kerr interaction on the scattering. The delta function corresponds to energy conservation, and leads to entanglement in frequency modes. The ideal CPHASE gate

is defined by conditions that single photon inputs remain untouched, with  $S_1^{\text{ideal}}(\omega_a; \nu_a) = \delta(\omega_a - \nu_a)$ , while two photon scattering leads to the accumulated phase shift  $\phi$  in the form  $S_2^{\text{ideal}}(\omega_a, \omega_b; \nu_a, \nu_b) = e^{i\phi} \delta(\omega_a - \nu_a) \delta(\omega_b - \nu_b)$ . Thus, we search for the condition for the two-photon state to become a product state, but adding the non-trivial conditioned phase. We note that in general there might be additional trivial phases added to each mode. This is especially true as in our case  $\omega_a \neq \omega_b$ . However, this corresponds to a single photon deformation that can be removed by performing additional individual rotations.

Having defined the necessary ingredients for the single node we proceed to the multi-node case of connected cavities. As noted before, only one-way propagation is considered, and two distinct cases arise: counter-propagating modes and co-propagating modes<sup>19</sup>. We follow the discussion in supplemental material of Ref.<sup>18</sup>, and write the  $N$ -site scattering matrix for counter-propagating modes as

$$S_1(\omega_a; \nu_a)^{(N)} = \left( -\frac{\Gamma^*(\omega_a)}{\Gamma(\omega_a)} \right)^N \delta(\omega_a - \nu_a), \quad (\text{S21})$$

and similar holds for the mode  $\hat{b}$ . The two-photon scattering matrix can be generalized as

$$S_2(\omega_a, \omega_b; \nu_a, \nu_b)^{(N)} = S_1(\omega_a; \nu_a)^{(N)} S_1(\omega_b; \nu_b)^{(N)} \quad (\text{S22})$$

$$- i \frac{\chi \gamma^2}{\pi} \left( 1 + \frac{2i\chi}{\Gamma(\omega_a) + \Gamma(\omega_b)} \right)^{-1} \frac{\delta(\omega_a + \omega_b - \nu_a - \nu_b)}{\Gamma(\omega_a)\Gamma(\omega_b)\Gamma(\nu_a)\Gamma(\nu_b)} \times$$

$$\times \left[ \sum_{j=1}^N \left( \frac{\Gamma^*(\omega_a)\Gamma^*(\nu_b)}{\Gamma(\omega_a)\Gamma(\nu_b)} \right)^{N-j} \left( \frac{\Gamma^*(\omega_b)\Gamma^*(\nu_a)}{\Gamma(\omega_b)\Gamma(\nu_a)} \right)^{j-1} \right].$$

Finally, the gate fidelity  $F$  of CPHASE operation can be derived through the average over possible input states, leading to  $F(\phi) = (6 + 3\text{Re}\{e^{i\phi} O^{(N)}\} + |O^{(N)}|^2)/10$ . Here we used the overlap between single and two-photon wavepackets that reads

$$O^{(N)} = \int d\nu_a d\nu_b d\omega_a d\omega_b d\omega'_a d\omega'_b \xi(\omega_a) \xi(\omega_b) \xi(\omega'_a) \xi(\omega'_b) \times \quad (\text{S23})$$

$$\times \left[ S_1^{(N)}(\omega_a, \nu_a) S_1^{(N)}(\omega_b, \nu_b) \right]^* S_2^{(N)}(\omega'_a, \omega'_b; \nu_a, \nu_b),$$

and is crucial for distinguishing the two-photon output from the product state.  $\xi(\omega; \sigma) \equiv \xi(\omega)$  is a standard Gaussian function parametrized by the frequency width  $\sigma$ , and we omit for simplicity underlying parameters. The overlap of  $O = -1$  corresponds to the perfect phase gate. The resulting gate fidelity can be easily calculated for various phase shift  $\phi$ .

We perform proof-of-principle calculation for counter-propagating modes, considering different parameters and number of nodes in the lattice  $N$ . To simplify the description, we consider a limiting case of  $N \rightarrow \infty$ . Then, we

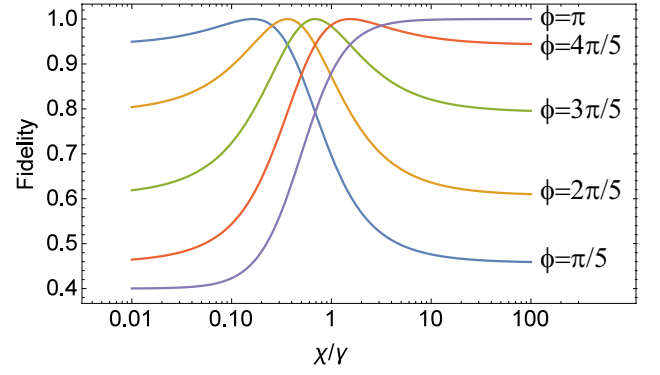

**Supplementary Figure 9.** Fidelity of CPHASE gate for different Kerr interaction strength ratio,  $\chi/\gamma$ , plotted for different phase  $\phi \in \{\pi/5, \pi\}$ . Results are for infinite limit of cavities  $N \rightarrow \infty$  (in practice  $N > 20$  gives high fidelity), and narrow pulses  $\sigma \rightarrow 0$ .

can write the two-photon scattering matrix as

$$S_2^{(\infty)}(\omega_a, \omega_b; \nu_a, \nu_b) = S_1^{(\infty)}(\omega_a, \nu_a) S_1^{(\infty)}(\omega_b, \nu_b) \left[ 1 - \frac{i\chi\gamma^3}{4} \left( 1 + \frac{2i\chi}{\Gamma(\omega_b) + \Gamma(\omega_a)} \right)^{-1} \frac{1}{|\Gamma(\omega_b)\Gamma(\omega_a)|^2} \right], \quad (\text{S24})$$

and further simplification is possible if we consider photons arriving on resonance,  $\omega \approx \Delta$ . From here we can plot the real part of the two-photon scattering matrix, that is equal to the product of single-photon matrices in the limit of  $\chi/\gamma \ll 1$  (overlap is equal to 1), and changes sign for  $\chi/\gamma \gg 1$ , leading to overlap of  $-1$ . The interplay of overlap value and target conditional phase thus determines  $F(\phi)$ . We plot the fidelity of the CPHASE gate as a function of  $\chi/\gamma$  in Supplementary Figure 9. We observe that while full  $\pi$ -phase gate may be difficult to get with smaller interaction constants, we can get high-fidelity for fractional  $\pi$  gates. Given that suitable universal gate set can be formed with these gates, we can conclude  $\chi/\gamma$  may work in the cascaded fashion. We can also infer the number of sites dependence for fidelity using scaling in Ref.<sup>18</sup>. This shows that fidelity rapidly improves with  $N$  and already at  $N = 10$  reaches 0.99 values.

## Supplementary Discussion 8. XPM for quantum computing: the outlook

We have shown that polaritonic micropillars with cross-Kerr interaction can be used to perform conditional phase shift on the signal mode induced by the control. Working with weak optical beams, the system can be used as a quantum nondemolition detector and exploited in sensing applications. Moreover, in the limiting case of single photon inputs for the signal and control modes the system enters the realm of quantum information processing applications. Performing single photon operations

in the current setup is difficult, and requires improvements outlined in the previous section. However, we aim to answer another important question: Is it *in principle* possible to perform quantum computing with polaritonic pillars in the lattice geometry?

In the preceding section we showed that using the polaritonic lattices and cascaded geometry the high-fidelity CPHASE gate for conditional angle  $\phi$  can be realized even in the case of weak nonlinearity  $\chi/\gamma < 1$ . This however favours small angle rotations  $\phi$  being a fraction of full  $\pi$ . We note that CPHASE gate for the condition phase shift of  $\phi$  corresponds to the unitary  $\exp[i\phi(\hat{Z}_1\hat{Z}_2 - \hat{Z}_1 - \hat{Z}_2)]$ , where  $\hat{Z}_{1,2}$  are Pauli Z matrices acting on photonic modes 1 and 2 (with restricted  $\{0, 1\}$  occupation)<sup>23</sup>. This unitary can be performed for the phase  $\varphi = \pi/m$  ( $m > 1$ ). Repeating the gate  $m$  times we can get the  $\pi$  shift (CZ gate). CZ can be converted to CNOT gate using conjugation by two Hadamard gates for one of the modes represented by simple photonic mode beam-splitters,  $\hat{U}_{12}^{\text{CNOT}} = \hat{H}_1 \hat{U}_{12}^{\text{CZ}} \hat{H}_1$ <sup>23</sup>. Together with single qubit rotations CNOT forms a universal gate set, and thus provides a toolbox for a universal quantum computation. However, we note that concatenation leads to the overall lower fidelity. Namely, as we chain gates based on the finite number of micropillars, the associated CPHASE infidelity  $(1 - F_\phi)$  is small but finite. Performing  $m$  gates in a row gives  $\propto (1 - F_\phi^m)$  infidelity scaling, and correspondingly restricts (from below) the number

of cavities needed for high-fidelity operation. Thus  $m$  cannot be large, dictating the substantial  $\chi/\gamma$  ratio. Ultimately, the remaining error related to finite size requires error correction (much like with any other quantum computing architectures), and finding the requirements of polaritonic setup in terms of the error-correction threshold is an important question for the future.

Finally, we suggest that the described polaritonic CPHASE operations can be used in the radically different way. Imagine the linear optical setup where optical signals are operated by beam-splitters, phase shifts, delays, and single qubit rotations<sup>24</sup>. This serves as a base to the boson sampling<sup>25,26</sup>, and was shown to be #P-hard problem. We also know that nonlinearity introduces complexity in the quantum circuits, staying behind universal speed-ups<sup>23</sup>. We suggest that polaritonic lattices and CPHASE gates can be used to inject entanglement in the otherwise linear networks. This can be seen as a resource for further computation, much like T gates used in Google's quantum supremacy experiment<sup>27</sup> with IQPs (instantaneous quantum polynomial-time circuits). Joining high fidelity linear operation and high-fidelity weakly nonlinear operation we can exploit the hybrid quantum-classical workflow, where CPHASE-induced entanglement is sculptured by single mode rotations with angles defined variationally. This has shown to be the preferred strategy for near-term quantum devices and represents an efficient workflow for designing quantum software<sup>28</sup>. In this case, polariton-based CPHASE gates offer a unique deterministic way to nonlinear operations.

- 
- <sup>1</sup> Whittaker, D. M. [Classical treatment of parametric processes in a strong-coupling planar microcavity](#). *Physical Review B* **63**, 193305 (2001).
  - <sup>2</sup> Becker, W. *The bh TCSPC Handbook* (Becker & Hickl GmbH, Berlin, Germany, 2019), 8th edn.
  - <sup>3</sup> Ismail, N., Kores, C. C., Gekus, D. & Pollnau, M. [Fabry-pérot resonator: spectral line shapes, generic and related airy distributions, linewidths, finesse, and performance at low or frequency-dependent reflectivity](#). *Optics Express* **24**, 16366 (2016).
  - <sup>4</sup> Diniz, I. *et al.* [Strongly coupling a cavity to inhomogeneous ensembles of emitters: Potential for long-lived solid-state quantum memories](#). *Physical Review A* **84**, 063810 (2011).
  - <sup>5</sup> Gehrsitz, S. *et al.* [The refractive index of Al<sub>x</sub>Ga<sub>1-x</sub>As below the band gap: Accurate determination and empirical modeling](#). *Journal of Applied Physics* **87**, 7825–7837 (2000).
  - <sup>6</sup> Aspnes, D. E., Kelso, S. M., Logan, R. A. & Bhat, R. [Optical properties of Al<sub>x</sub>Ga<sub>1-x</sub>As](#). *Journal of Applied Physics* **60**, 754–767 (1986).
  - <sup>7</sup> Born, M. & Wolf, E. *Principles of optics: electromagnetic theory of propagation, interference and diffraction of light; 2nd ed.* (Pergamon, Oxford, 1964).
  - <sup>8</sup> Vorobyev, O. B. [Energy density of macroscopic electric and magnetic fields in dispersive medium with losses](#). *Progress In Electromagnetics Research B* **40**, 343–360 (2012).
  - <sup>9</sup> Landau, L. D. & Lifshitz, E. [The electromagnetic wave equations](#). In *Electrodynamics of Continuous Media*, 257–289 (Elsevier, 1984).
  - <sup>10</sup> Loudon, R. [The propagation of electromagnetic energy through an absorbing dielectric](#). *Journal of Physics A: General Physics* **3**, 450–450 (1970).
  - <sup>11</sup> Zheng, X. & Palfy-Muhoray, P. [Electrical energy storage and dissipation in materials](#). *Physics Letters A* **379**, 1853–1856 (2015).
  - <sup>12</sup> Delteil, A. *et al.* [Towards polariton blockade of confined exciton–polaritons](#). *Nature Materials* **18**, 219–222 (2019).
  - <sup>13</sup> Renucci, P. *et al.* [Microcavity polariton spin quantum beats without a magnetic field: A manifestation of coulomb exchange in dense and polarized polariton systems](#). *Phys. Rev. B* **72**, 075317 (2005).
  - <sup>14</sup> Shapiro, J. H. [Single-photon kerr nonlinearities do not help quantum computation](#). *Physical Review A* **73**, 062305 (2006).
  - <sup>15</sup> Gea-Banacloche, J. [Impossibility of large phase shifts via the giant kerr effect with single-photon wave packets](#). *Phys. Rev. A* **81**, 043823 (2010).
  - <sup>16</sup> Fan, B. *et al.* [Breakdown of the cross-kerr scheme for photon counting](#). *Phys. Rev. Lett.* **110**, 053601 (2013).
  - <sup>17</sup> Chudzicki, C., Chuang, I. L. & Shapiro, J. H. [Deterministic and cascaded conditional phase gate for photonic qubits](#). *Physical Review A* **87**, 042325 (2013).
  - <sup>18</sup> Brod, D. J. & Combes, J. [Passive cphase gate via cross-kerr nonlinearities](#). *Phys. Rev. Lett.* **117**, 080502 (2016).

- <sup>19</sup> Brod, D. J., Combes, J. & Gea-Banacloche, J. Two photons co- and counterpropagating through  $N$  cross-Kerr sites. *Physical Review A* **94**, 023833 (2016).
- <sup>20</sup> Whittaker, C. E. *et al.* Exciton polaritons in a two-dimensional lieb lattice with spin-orbit coupling. *Phys. Rev. Lett.* **120**, 097401 (2018).
- <sup>21</sup> Klemmt, S. *et al.* Exciton-polariton topological insulator. *Nature* **562**, 552–556 (2018).
- <sup>22</sup> Combes, J., Kerckhoff, J. & Sarovar, M. The SLH framework for modeling quantum input-output networks. *Advances in Physics: X* **2**, 784–888 (2017).
- <sup>23</sup> Nielsen, M. A. & Chuang, I. L. *Quantum Computation and Quantum Information* (Cambridge University Press, 2000).
- <sup>24</sup> Kok, P. *et al.* Linear optical quantum computing with photonic qubits. *Rev. Mod. Phys.* **79**, 135–174 (2007).
- <sup>25</sup> Aaronson, S. & Arkhipov, A. The computational complexity of linear optics. *Theory of Computing* **9**, 143–252 (2013).
- <sup>26</sup> Wang, H. *et al.* Boson sampling with 20 input photons and a 60-mode interferometer in a  $10^{14}$ -dimensional hilbert space. *Phys. Rev. Lett.* **123**, 250503 (2019).
- <sup>27</sup> Arute, F. *et al.* Quantum supremacy using a programmable superconducting processor. *Nature* **574**, 505–510 (2019).
- <sup>28</sup> Benedetti, M., Lloyd, E., Sack, S. & Fiorentini, M. Parameterized quantum circuits as machine learning models. *Quantum Science and Technology* **4**, 043001 (2019).
